# Supplementary material for: Type I superconductivity in the Dirac semimetal PdTe2
Source: arXiv:1710.03862 source file (2017-10-11)
Supplement: Supplementary file 1 [file Supplemental_Material_Leng.pdf]

**SUPPLEMENTAL MATERIAL**

# Type I superconductivity in the Dirac semimetal $PdTe_2$

H. Leng[1], C. Paulsen[2], Y. K. Huang[1] and A. de Visser[1]

[1]*Van der Waals - Zeeman Institute, University of Amsterdam,*
*Science Park 904, 1098 XH Amsterdam, The Netherlands*
[2]*Institut Néel, CNRS & Université Grenoble Alpes, BP 166, 38042 Grenoble, France*

**Content**

1. SEM and EDX

2. Demagnetization factor

3. Ac-susceptibility: dependence on the ac-driving field $H_{ac}$

4. Resistance measurements

5. Field-depression of superconductivity measured by resistance

6. Superconducting phase diagram determined by resistance

7. Dc-magnetization and ac-susceptibility after polishing the crystal surfaces

8. Superconducting phase diagram after polishing

## 1. SEM and EDX

The chemical composition and stoichiometry of the prepared $PdTe_2$ crystal was investigated by Scanning Electron Microscope (FEI Verios 460) with Electrons Dispersive X-ray Spectroscopy at the Institute AMOLF (Amsterdam). Experiments were made on several single-crystalline pieces, some of them with freshly cleaved surfaces. A typical SEM micrograph and composition layout is shown in Fig S1. We did not detect any inhomogeneities or impurity phases. The measured Pd:Te ratio is 1:2 within the experimental resolution of 0.5 %.

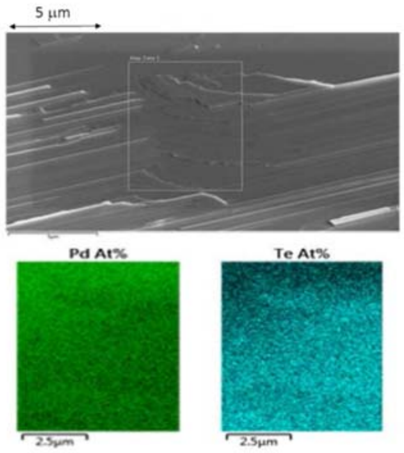


*Fig. S1 SEM picture and EDX mapping of Pd and Te.*

## 2. Demagnetization factor

The dimensions and shape of the $PdTe_2$ crystal used for the magnetization measurements are reported in Fig. S2. The magnetic field was applied along the long direction (*a*-axis). In order to estimate the demagnetization factor, $N$, we approximated the shape by a bar with dimensions $4.4\times1.6\times0.65$ mm$^3$. We calculate $N = 0.10$ (see Chen *et al*., IEEE Transactions on Magnetics **38** 1742, 2002).

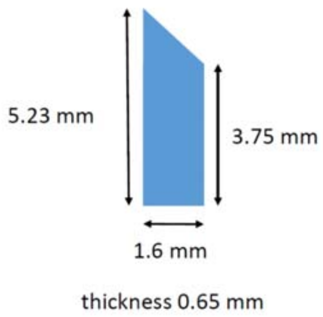


*Fig. S2 Dimensions and shape of the $PdTe_2$ single crystal s2.*

### 3. Ac-susceptibility: dependence on the ac-driving field $H_{ac}$

In Fig. S3a we show the low frequency ac-susceptibility of $PdTe_2$ (crystal s2) at $T = 0.60$ K as a function of applied field, $H_a$, measured for 5 different amplitudes of the ac-driving field, $H_{ac}$. For the largest amplitude, $\mu_0 H_{ac} = 0.25$ mT, the peak due to the differential paramagnetic effect (DPE) below $H_c$ is very pronounced. For fields $H > H_c(0.6K) = 12$ mT a diamagnetic signal is still visible. Upon reducing the amplitude of $H_{ac}$ the extra diamagnetic signal grows progressively and screens the peak due to the DPE more and more. For the lowest amplitude of the ac-driving field, $\mu_0 H_{ac} = 0.0005$ mT, the DPE peak is completely screened and a full screening signal (100 % sample volume) persists till 14 mT. This can only be caused by superconductivity of the surface layer (which is present already below $H_c$). For higher applied fields flux penetrates the crystal in a step-wise fashion, which indicates an intricate flux pinning process at the surface. Flux penetrates more easily when the amplitude of $H_{ac}$ is increased. In Fig. S3b we show the field variation $\chi_{ac}'(H_a)$ for $\mu_0 H_{ac} = 0.005$ mT at different temperatures. Here the driving field is 10 times larger than $H_{ac}$ used to take the data presented in Fig. 3d in the manuscript. The weaker screening in Fig. S3b is obvious and the DPE peak remains visible even at the lowest temperature. From our ac-susceptibility study we conclude that superconductivity of the surface layer accompanies bulk superconductivity. The efficacy of the surface layer to pin flux strongly depends on the amplitude of the ac-driving field, and is already strongly reduced for $\mu_0 H_{ac}$ = 0.25 mT.

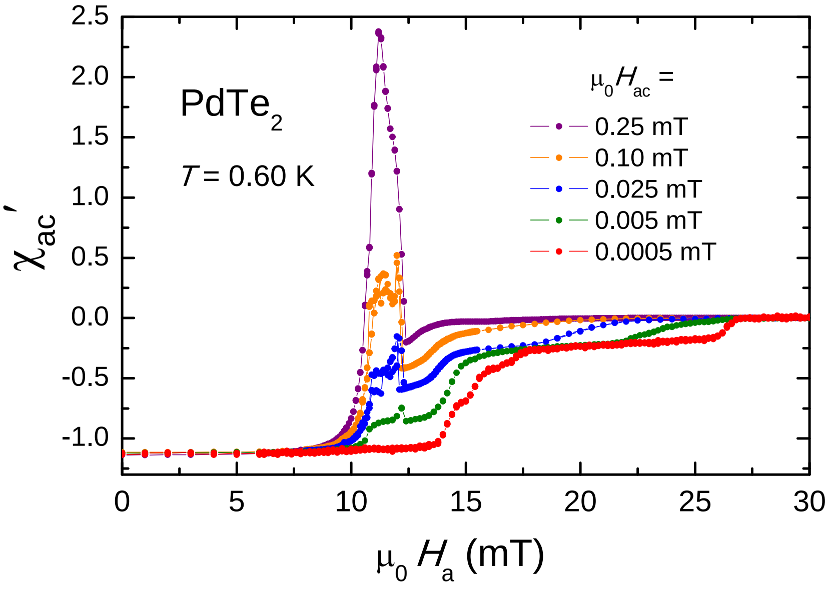


*Fig. S3a Ac-susceptibility of $PdTe_2$ (crystal 2) at $T = 0.60$ K as a function of the applied field, $H_a$, in driving fields, $\mu_0 H_{ac}$, ranging from 0.0005 mT to 0.25 mT as indicated.*

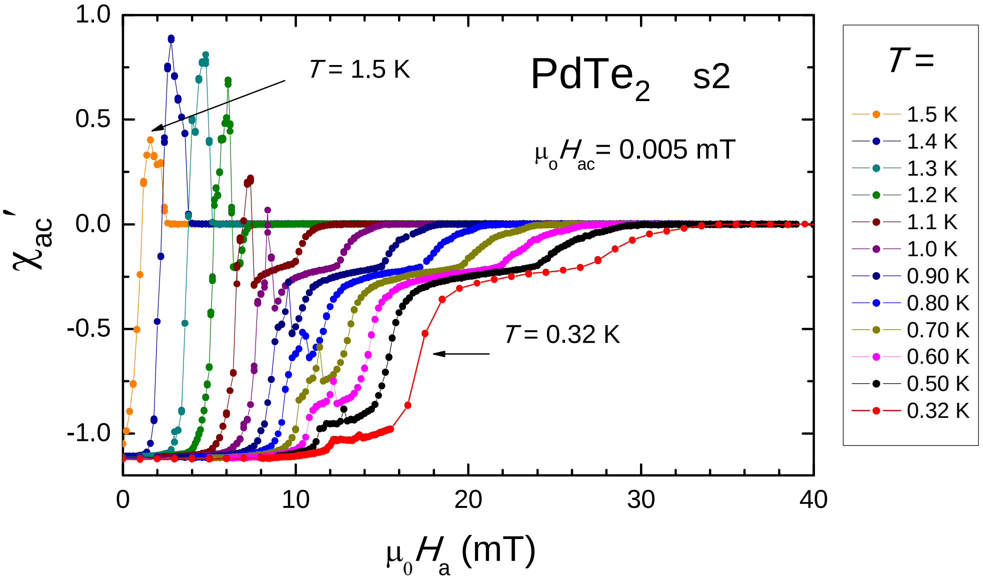


*Fig. S3b Ac-susceptibility of $PdTe_2$ (crystal 2) as a function of the applied field, $H_a$, in a driving fields $\mu_0 H_{ac}$ = 0.005 mT at temperatures in the range T = 0.32-1.5 K as indicated. Here $H_{ac}$ is 10× larger than in Fig. 3d in the manuscript.*

## 4. Resistance measurements

For the electrical resistivity measurements current and voltage contacts were made by attaching thin copper wires in a four-point configuration on the bar-shaped crystals by silver paste. The electrical resistivity, ρ(*T*), was measured in the PPMS in the temperature range 2-300 K for a current ($I$ = 1 mA) in the basal plane, see Fig. S4. The overall temperature variation ρ(*T*) is in agreement with the data reported by Hooda and Yadav (e-print arXiv:1704.07194v1), but the absolute ρ-value at room temperature (23 μΩcm) is a factor 2 smaller in our case. Wang *et al.*, (Sci. Rep. 6, 31554, 2016) presented a similar ρ(*T*)-curve, but with much larger absolute values. The residual resistance ratio, RRR=*R*(300K)/*R*(2K) amounts to 30. In the inset we show the superconducting transition measured in the 3-He refrigerator (Heliox, Oxford Instruments). In the Heliox the resistance was measured by a Linear Research 700 bridge, using a low-frequency ac-method and an excitation current of 1 mA.

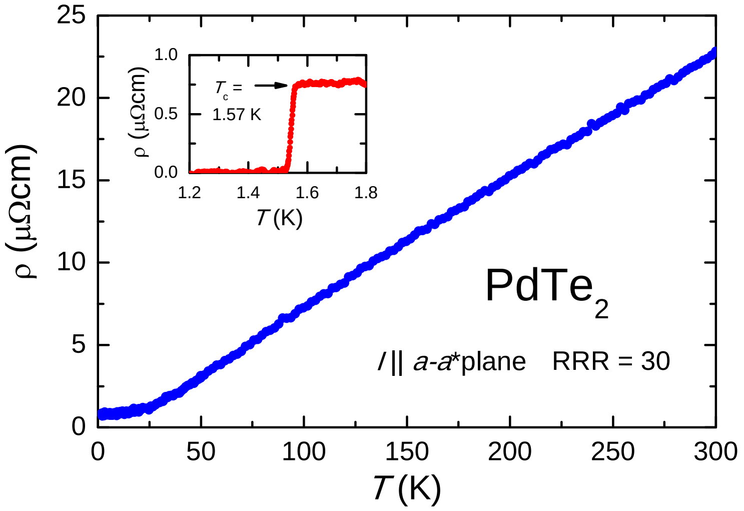


*Fig. S4 Temperature variation of the electrical resistivity of* $PdTe_2$*. The inset shows the superconducting transition. The arrow points to the onset temperature* $T_c^{onset}$ *of 1.57 K.*

## 5. Field-depression of superconductivity measured by resistance

The depression of superconductivity in $PdTe_2$ (crystal 2) was studied by measuring the resistance, $R(T)$, in fixed magnetic fields applied along the *a*-, *a**- and *c*-axis. Data for $H_a \parallel a$ are taken in the longitudinal configuration ($H_a \parallel I$), while data for $H_a \parallel a^*$ and $H_a \parallel c$ are taken in the transverse configuration ($H_a \perp I$). In Figs. S5a and S5b we present the data for $H_a \parallel a^*$ and $H_a \parallel a$, respectively. Since the critical field for the Type I superconducting phase is low ($H_c$ = 13.6 mT for $T \rightarrow 0$), special care was taken to reduce the remanent field in the superconducting magnet to close to zero (by reversing the field polarity while sweeping the field to zero) in the experiment for $H_a \parallel a^*$. The data for $H_a \parallel a^*$ show a sharp superconducting transition in the low field range (up to 4 mT), *i.e.* when the phase boundary of Type I superconductivity is probed (see inset Fig. S6). In higher applied fields the transition broadens gradually and superconductivity is depressed less rapidly. The measured $R(T)$-curves for $H_a \parallel c$ (not shown) are comparable to the ones for $H_a \parallel a$. The field-depression of superconductivity was also measured on two other crystals with similar results.

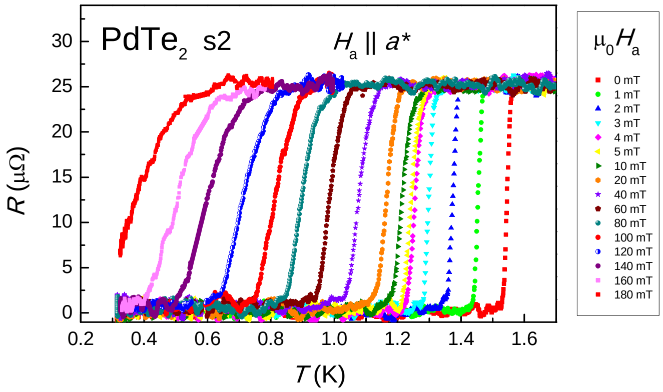


*Fig. S5a Temperature variation of the resistance of $PdTe_2$ (crystal 2) measured in fixed applied magnetic fields $H_a \parallel a^*$ as indicated.*

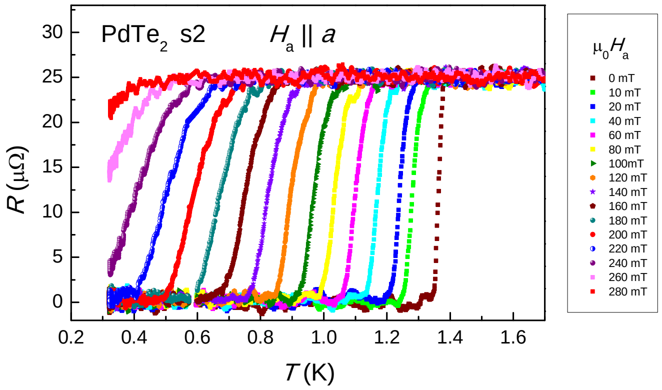


*Fig. S5b Temperature variation of the resistance of $PdTe_2$ (crystal 2) in fixed fields $H_a \parallel a$ as indicated. We remark, in this experiment the field values are not corrected for the small remanent field of about 3 mT present in the superconducting magnet.*

## 6. Superconducting phase diagram determined by resistance

By collecting the transition temperatures measured at fixed fields in the $H_a$-$T$ plane we construct the superconducting phase diagram determined by resistance shown in Fig. S6. Here we use the onset $T_c$ for superconductivity. We remark that by defining $T_c$ as the midpoint of the transition or at $R = 0$ the $T_c$ values will be reduced to some degree, but this will not affect the main features of the diagram. In very low fields (up to 4 mT) we observe the depression of the bulk Type I superconducting phase (see inset in the left panel). However, superconductivity survives up to much larger fields. For $H_a \parallel a$ we find a critical field $\mu_0 H_c^R \approx 0.3$ T for $T \rightarrow 0$ (see manuscript). We attribute the $R = 0$ state for fields exceeding 4 mT to superconductivity of the surface (see manuscript). The $H_c^R(T)$-curves are remarkably isotropic with respect to the direction of the magnetic field. This rules out a scenario of filamentary superconductivity with filaments in the planes of the layered material. In this case one expects to observe a large anisotropy of $H_c^R(T)$ for a field along and perpendicular to the $c$-axis. The presence of filaments perpendicular to the layer direction is highly unlikely. In the right panel of Fig. S6 we have traced the $H_c^R(T)$-data in a "universal" reduced plot $b(t)$, where $b = H_c^R(T) /[-(dH_c^R/dT)|_{Tc} \times T_c]$ and $t = T/T_c$. Here we take $T_c = T_c^s = 1.33$ K. The data compare well with the Werthamer-Helfand-Hohenberg model curve for an orbital-limited weak-coupling spin-singlet superconductor in the clean limit (Werthamer *et al.*, Phys. Rev. **147**, 295, 1966).

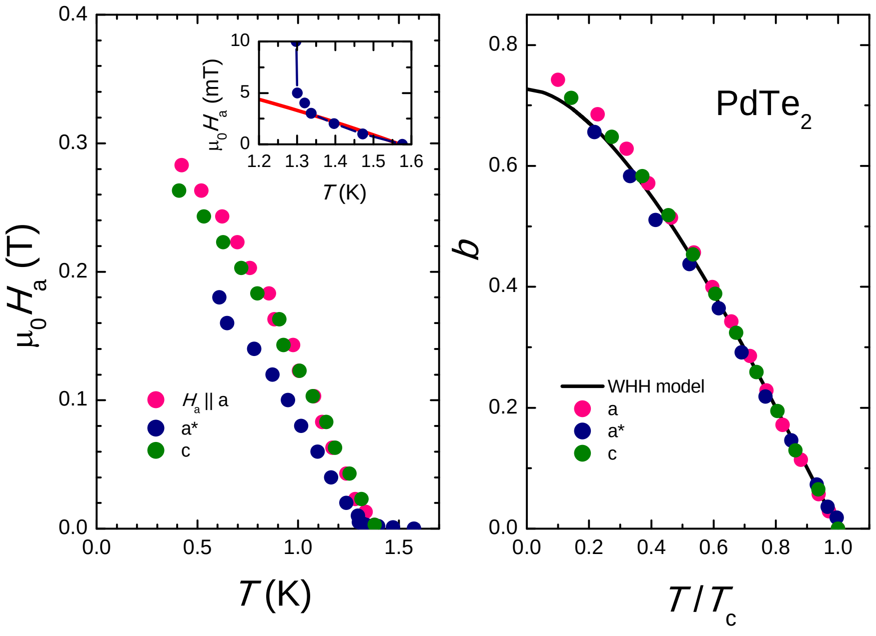


*Fig. S6 Left panel: Field-temperature phase diagram of superconductivity in $PdTe_2$ (crystal 2) measured by resistance. Data points are taken from $T_c^{onset}$ in the R(T)-curves measured at fixed fields. The inset shows low-field data for $H_a$ || a* that initially follow the $T^2$-variation of $H_c(T)$ (red line). Right panel: Reduced critical field, $b = H_c^R(T) /[-(dH_c^R/dT)|_{Tc} \times T_c]$ as a function of the reduced temperature $T/T_c$. The data are compared to the WHH model curve (black line).*

**7. Dc-magnetization and ac-susceptibility after polishing the crystal surfaces**

The bar-shaped $PdTe_2$ crystal used for the magnetization study was cut from a bigger piece by a scalpel blade. The cuts along the *ac*-plane were made by spark erosion. In order to exclude that surface superconductivity is due to an impurity face due to the defected spark-cut layer, the crystal's surfaces were carefully polished by 3 and 1 μm diamond paste till the surfaces appeared brilliant. Next, the dc-magnetization and ac-susceptibility measurements were repeated on the polished crystal. The results basically show that superconductivity of the surface sheath is not removed by polishing. In Fig. S7a we show the dc-magnetization. The data are close to identical to the data reported in Fig. 1 in the manuscript. The tail in $M(H)$ for $H_a > H_c$, which is a signature of surface superconductivity, is reproduced. In Fig. S7b we show the dc-magnetization, or rather $M/H_a$, as a function of temperature. Again the data are essentially identical to the data reported in Fig. 2 in the manuscript. Also, the amount of expulsed flux decreases for the lowest dc-fields (0.10 and 0.01 mT). This was attributed to the weak pinning capability of the surface layer. In Figs. S7c and S7d we report ac-susceptibility measurements as a function of field in driving fields of 0.25 mT and 0.0005 mT, respectively. The latter data-set shows that the screening due to the surface is less effective compared to the data taken before polishing (Fig. 3d in the manuscript). It indicates the polished surface is less effective in pinning the flux. On the other hand surface superconductivity persists to higher fields: 44 mT for the polished sample compared to 33 mT before polishing (at the lowest temperature of 0.31 K).

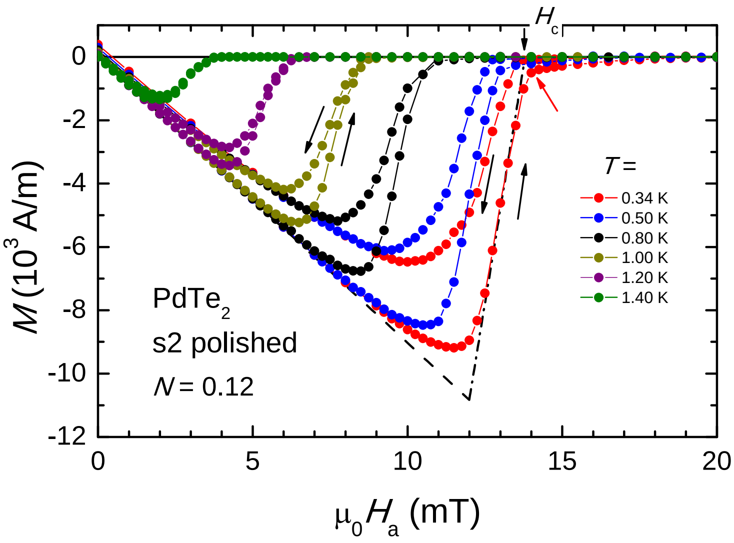


*Fig. S7a ZFC and FC dc-magnetization per unit volume as a function of applied field for $PdTe_2$ crystal 2 after polishing at temperatures from 0.34 K (right) to 1.4 K (left) as indicated. The initial slope $\chi_m = dM/dH_a$ accounts for a superconducting sample volume of 100 % with N = 0.12 (dashed line). The dash-dotted line indicates the idealized $M(H_a)$-curve with slope 1/N in the intermediate state at T = 0.34 K. The red arrow points to the start of a tail in $M(H_a)$ indicating surface superconductivity.*

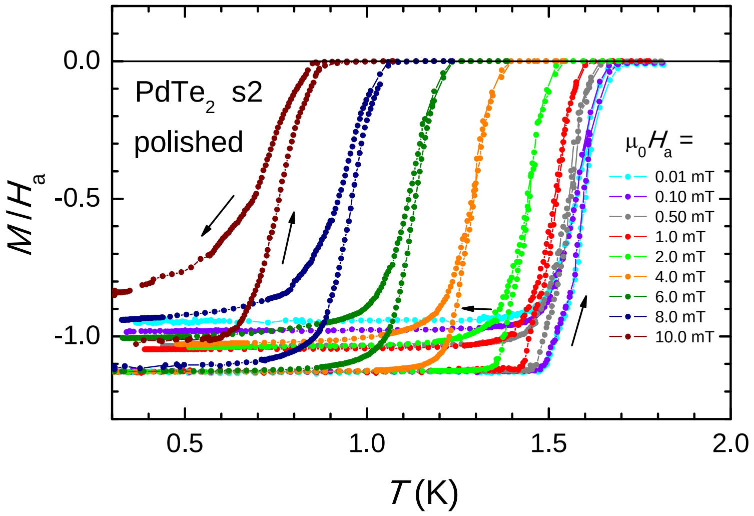


*Fig. S7b ZFC-FC dc-susceptibility, $M/H_a$, in S.I. units, as a function of temperature in fields $\mu_0 H_a$ from 0.01 mT (right) to 10.0 mT (left) as indicated. The data are taken on $PdTe_2$ crystal 2 after polishing.*

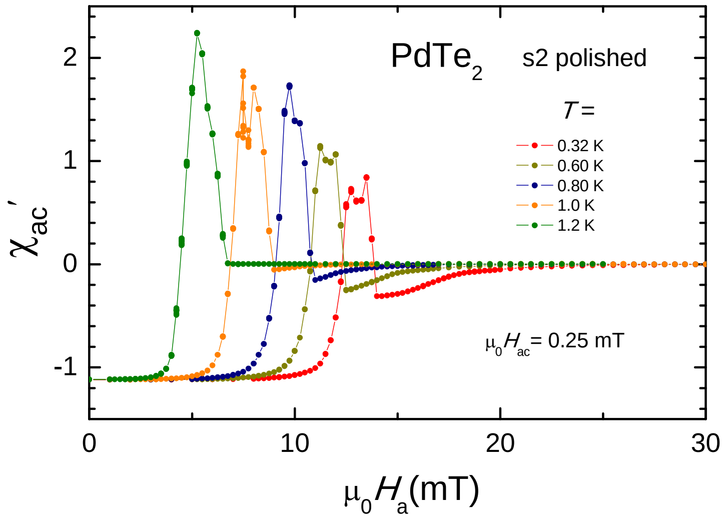


*Fig. S7c Ac-susceptibility as a function of applied field of $PdTe_2$ crystal 2 after polishing. The driving field $\mu_0 H_{ac}$ = 0.005 mT. Data are taken at temperatures from 0.32 K to 1.2 K as indicated. The diamagnetic contribution above the DPE peak, i.e. for fields $H_a > H_c$, signals surface superconductivity.*

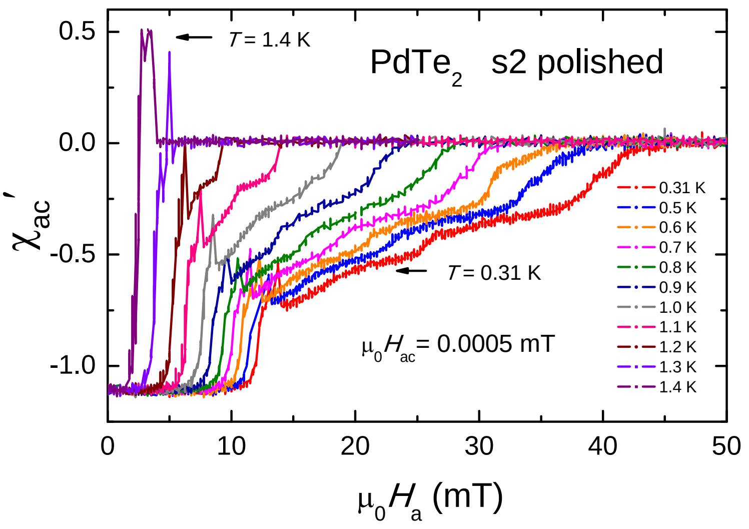


*Fig. S7d Ac-susceptibility of $PdTe_2$ crystal 2 after polishing as a function of the applied field. Data were taken in a driving field $\mu_0 H_{ac}$ = 0.0005 mT at temperatures in the range T = 0.31-1.4 K as indicated.*

### 8. Superconducting phase diagram after polishing

In Fig. S8 we present the superconducting phase diagram for the polished $PdTe_2$ crystal. The data points are collected from dc-magnetization (Figs. S7a and S7b) and ac-susceptibility (Figs. S7c and S7d). The phase boundary for surface superconductivity, $H_c^s(T)$, is obtained by identifying the field where $\chi_{ac}'$ loses its diamagnetic character ($\chi_{ac}' = 0$), see Fig. S7d. Here we used the $\chi_{ac}'$-data measured with the lowest amplitude of the ac-driving field $\mu_0 H_{ac} = 0.0005$ mT. The $H_c^s(T)$-curve lies above the curve reported in Fig. 4 in the manuscript. After polishing $\mu_0 H_c^s(0) = 46.2$ mT, compared to $\mu_0 H_c^s(0) = 34.9$ mT before polishing. The values of $T_c^s$ obtained by extrapolating $H_c^s(T)$ to zero field in the unpolished and polished case are identical within the error bar. We remark that the value of $H_c^s(0)$ depends on the amplitude of the ac-driving field, and that there are subtle effects of polishing on the pinning ability of the surface layer. But overall, the phase diagram before and after polishing is the same. We did not measure the $H_c^R$ phase boundary by resistance on the $PdTe_2$ crystal 2 after polishing. However, resistance measurements on two other crystals with freshly cleaved surfaces confirmed enhanced values $H_c^R$ >> $H_c$.

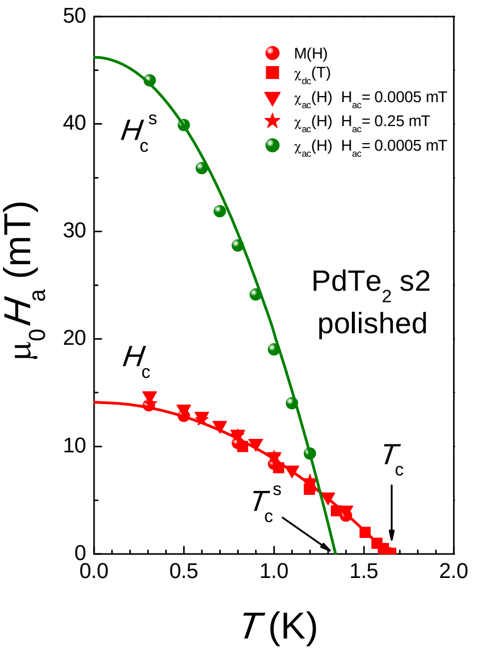


*Fig. S8 Superconducting phase diagram of $PdTe_2$ crystal 2 after polishing. Data points are taken from dc-magnetization and ac-susceptibility as indicated. The solid red and green lines represent fits to the critical fields $H_c$ for bulk superconductivity and $H_c^s$ for surface superconductivity with a quadratic temperature function (see manuscript).*
